# Supplementary material for: Masked LoGoNet: Fast and Accurate 3D Image Analysis for Medical Domain
Source: arXiv:2402.06190 source file (2025-03-28)
Supplement: Supplementary file 1 [file BTCV_res_images.tex]

\begin{figure*}[ht]
  \centering
  \begin{tabular}{c|cccccc}
   \hline
    {Ground Truth} & \textbf{LoGoNet} & DiNTS Search & SwinUNETR48 & UNet++ & Attention U-Net \\
    \hline
    \includegraphics[width=2.65cm]{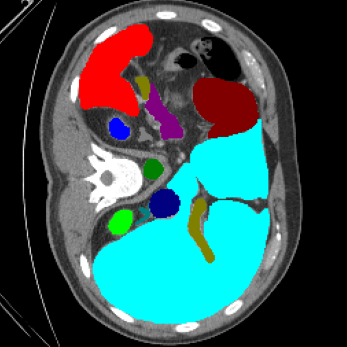} &
    \includegraphics[width=2.65cm]{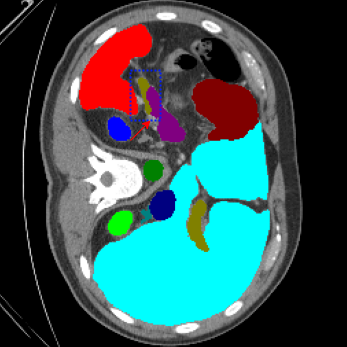} &
    \includegraphics[width=2.65cm]{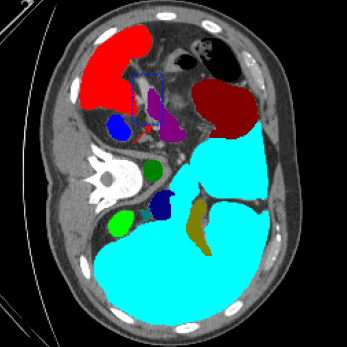} &
    \includegraphics[width=2.65cm]{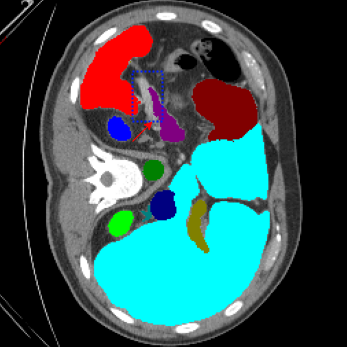} &
    \includegraphics[width=2.65cm]{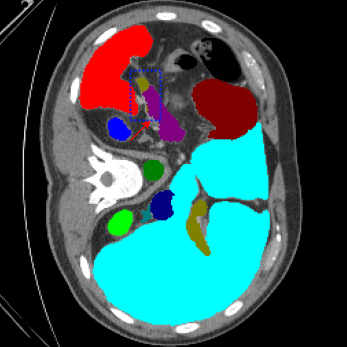} &
    \includegraphics[width=2.65cm]{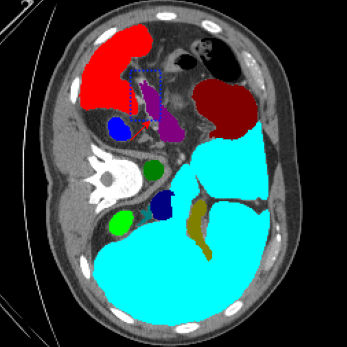} \\

    % \cline{2-7}
    \includegraphics[width=2.65cm]{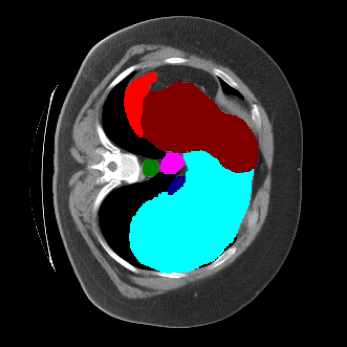} &
    \includegraphics[width=2.65cm]{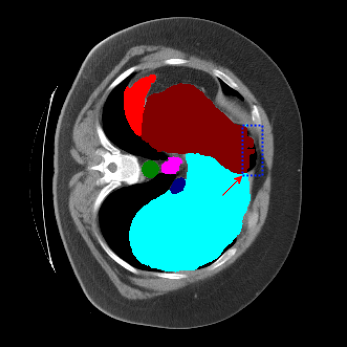} &
    \includegraphics[width=2.65cm]{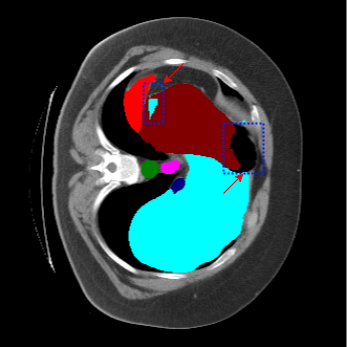} &
    \includegraphics[width=2.65cm]{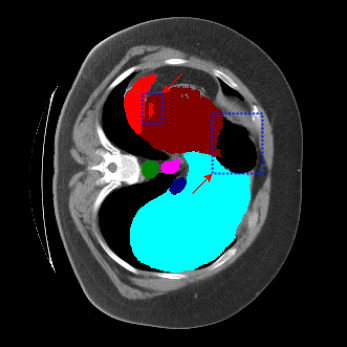} &
    \includegraphics[width=2.65cm]{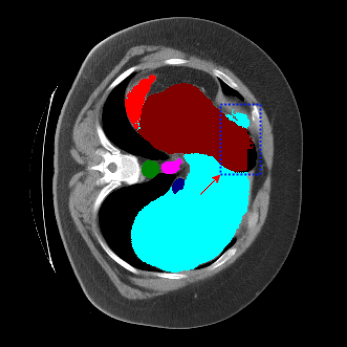} &
    \includegraphics[width=2.65cm]{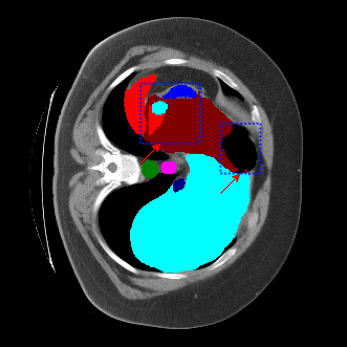} \\

    % \cline{2-7}
    \includegraphics[width=2.65cm]{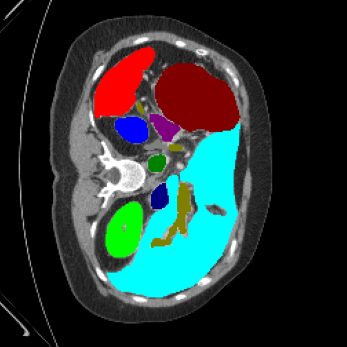} &
    \includegraphics[width=2.65cm]{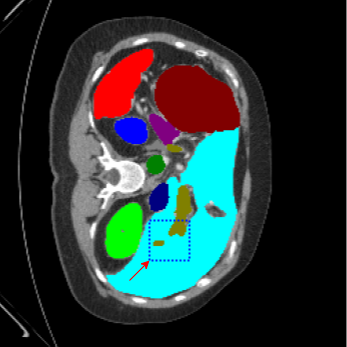} &
    \includegraphics[width=2.65cm]{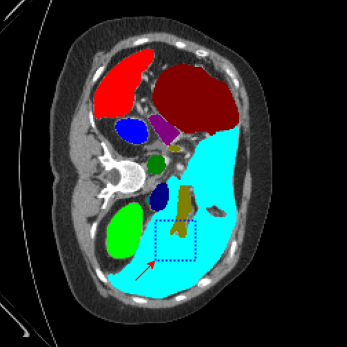} &
    \includegraphics[width=2.65cm]{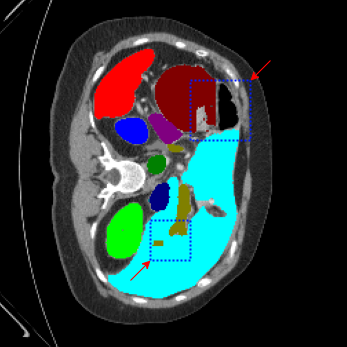} &
    \includegraphics[width=2.65cm]{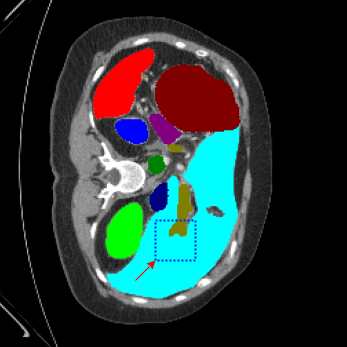} &
    \includegraphics[width=2.65cm]{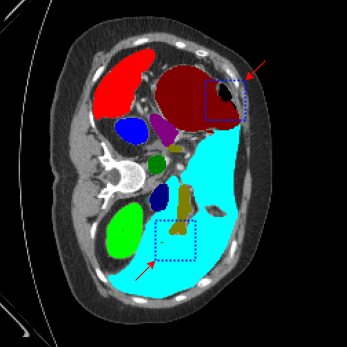} \\
    % \hline
    % \cline{2-7}

    \includegraphics[width=2.65cm]{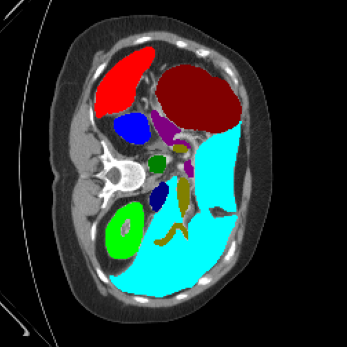} &
    \includegraphics[width=2.65cm]{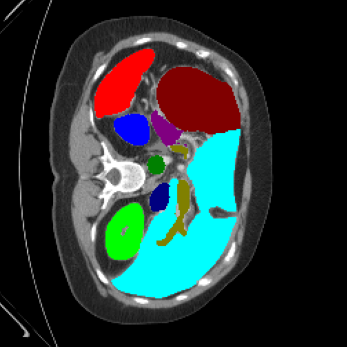} &
    \includegraphics[width=2.65cm]{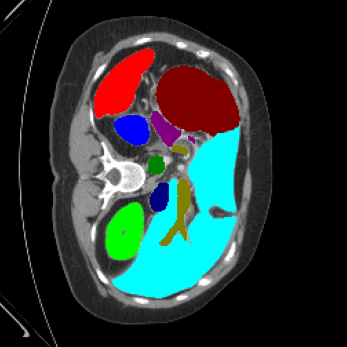} &
    \includegraphics[width=2.65cm]{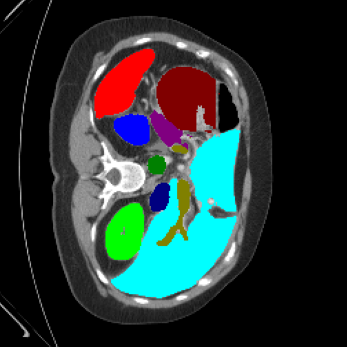} &
    \includegraphics[width=2.65cm]{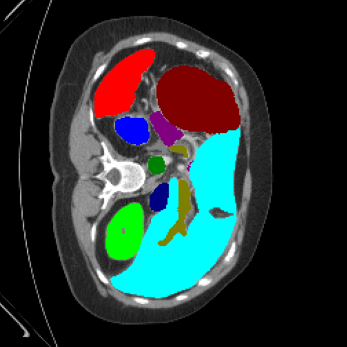} &
    \includegraphics[width=2.65cm]{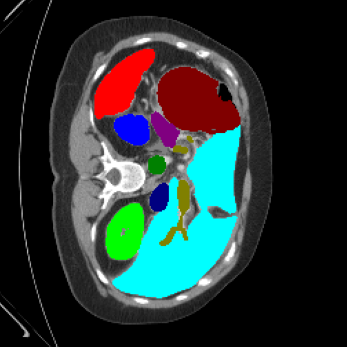} \\
    \hline
    % \cline{2-7}
  \end{tabular}
  \caption{A visualization of LoGoNet outputs compared to the output of the baseline models. Our model outperforms the baselines, particularly in the segmentation of small organ sections.}
  \label{fig:BTCV_res_app}
\end{figure*}
