# Supplementary material for: Masked LoGoNet: Fast and Accurate 3D Image Analysis for Medical Domain
Source: arXiv:2402.06190 source file (2025-03-28)
Supplement: Supplementary file 2 [file msd_res.tex]

\begin{table*}[ht]
\centering
\begin{tabular}{c|c|c|c|c|c|c}
Task & Colon Cancer & Spleen & Hepatic Vessels & Pancreas Tumour & Lung Tumours & Cardiac \\ \hline
SegResNetVAE & .742 & .968 & .745 & .740 & .765 & .951 \\
SwinUNETR48 & .695 & .967 & .737 & .738 & .763 & .957 \\
UNETR32 & .677 & .969 & .715 & .699 & .730 & .953 \\
UNet++ & .553 & .975 & .752 & .760 & .753 & .961 \\
nnUNet & .736 & .977 & .742 & .742 & .816 & .958 \\
DiNTS Search & .776 & \textbf{.980} & .749 & .749 & .768 & .960 \\
DiNTS Instance & .768 & .979 & .731 & .742 & .790 & \textbf{.963} \\
\textbf{ULKANet S} & .773 & .976 & .730 & .768 & .788 & .942 \\
\textbf{LoGoNet S} & \textbf{.786} & \textbf{.980} & \textbf{.757} & \textbf{.798} & \textbf{.802} & .951 \\ \hline
\textbf{ULKANet S + SSL} & {\ul .809} & {\ul .980} & .776 & {\ul .834} & .826 & .954 \\
\textbf{LoGoNet S + SSL} & .801 & {\ul .980} & {\ul .779} & .833 & {\ul .828} & {\ul .958}
\end{tabular}
  \caption{Result of the MSD dataset with  six different tasks based on Dice metric}
  \label{tab:MSD_res_app}
\end{table*}
